# Supplementary material for: PDP: Physics-Based Character Animation via Diffusion Policy
Source: arXiv:2406.00960 source file (2024-12-04)
Supplement: Supplementary file 1 [file appendix.tex]

\appendix
\section{Hyper-parameters}
% In this section, we detail hyper-parameters used for reproducability of the Diffusion Policy and the RL trained experts.

\subsection{PDP}
\begin{table}[H]
\label{tab:hyperparameter diffusion policy}
\begin{center}
\begin{tabular}{l | l | l}
  \toprule
  PDP Hyper-parameters   & AMASS tasks & Bump-em task  \\ \midrule
  Transformer Dim        & 512     & 256     \\
  Num Heads              & 8       & 8       \\
  Num Layers             & 10      & 8       \\
  Attention Dropout      & 0.3    & 0.3   \\
  \hline
  Optimizer              & \multicolumn{2}{c}{AdamW}   \\
  Weight Decay              & \multicolumn{2}{c}{1e-3}     \\
  Learning Rate          & \multicolumn{2}{c}{1e-4}    \\
  Learning Rate Warm-up: & \multicolumn{2}{c}{1000}   \\
  $\beta$-schedule       & \multicolumn{2}{c}{cosine}  \\
  Diffusion Steps        & \multicolumn{2}{c}{100}     \\
  \bottomrule
\end{tabular}
\end{center}
\bigskip\centering
\end{table}

\subsection{Expert Tracking Policies}
\begin{table}[H]
\label{tab:Expert Tracking Policies}
\begin{center}
\small\begin{tabular}{l | l | l}
  \toprule
  Tracking Policy Hyper-parameters   & AMASS tasks & Bump-em task  \\ \midrule
  Simulator                     & Isaac Lab & Mujoco    \\
  Optimizer                     & Adam      & AdamW     \\ 
  Actor Learning Rate          & 2e-5       & 1e-5      \\
  Critic Learning Rate         & 2e-5        & 1e-4     \\
  Exploration noise         & .055            & .082    \\
    
  Num Envs               & 500            & 100         \\ 
  Horizon Length         & 32             & 50          \\
  Mini-epochs            & 6              & 10          \\
  Batch size             & 16000          & 1250        \\

  Actor Hidden Layers           & [1024,512]     & [1024, 1024] \\
  Critic Hidden Layers    & [1024,512]     & [128, 128]   \\

  \hline
  $\gamma$             & \multicolumn{2}{c}{.99}   \\
  $\lambda$              & \multicolumn{2}{c}{.95}     \\
  clip               & \multicolumn{2}{c}{.2}    \\

  \bottomrule
\end{tabular}
\end{center}
\bigskip\centering
\end{table}
